# Supplementary material for: Monte Carlo goodness-of-fit tests for degree corrected and related stochastic blockmodels
Source: arXiv:1612.06040 source file (2024-03-06)
Supplement: Supplementary file 1 [file secAppendixV3asSECTION.tex]

\section*{Appendix A: Algebraic and geometric proofs of structure of the ER-SBM model}

%This section describes the ER-SBM polytope and Markov basis. 

Theorem A.1. is identical to Theorem  5.2, stated here for completeness. %\ref{thm: ER-SBM polytope} 
It gives an explicit description of the $H$-representation of the model polytope for the standard stochastic blockmodel, the ER-SBM. 

\smallskip 
%---THEOREM: ER-SBM Polytope----
%\begin{theorem}
\noindent{\bf Theorem A.1. [Theorem 5.2.]}
%\label{thm: ER-SBM polytope}
\emph{
Let $\M_{\mathrm{ER}}$ be an ER-SBM with node set $[n]$ partitioned into nonempty blocks $\B := \{B_1,\ldots,B_k\}$, and let $n_i:=|B_i|$ for all $i\in[k]$.  
Then the model polytope $P_{\M_{\mathrm{ER}}}$ is the ${k+1\choose 2}$-dimensional box
$$
\prod_{i\neq j}\left[0,n_in_j\right]\times\prod_{i=1}^k\left[0,{n_i\choose 2}\right].
$$
In particular, $P_{\M_{\mathrm{ER}}}$ is the intersection of the closed halfspaces given by the set of inequalities
\begin{equation*}
\begin{split}
0\leq &x_{ij} \leq n_in_j, \mbox{ for $1\leq i < j\leq k$, and}\\
0\leq &x_{ii} \leq {n_i\choose 2}, \mbox{ for $i\in[k]$}.\\
\end{split}
\end{equation*}
}
%\end{theorem}

\begin{proof} %[Proof of Theorem 4.1] %\ref{thm: ER-SBM polytope}]
Let $P$ denote the rectangle specified in the above theorem.  
Notice first that each vertex of the rectangle $P$ is clearly the sufficient statistics of some graph $g$.  
Thus, it suffices to show that $P_{\M_{\mathrm{ER}}}\subseteq P$.  
However, this is also easy to see by considering the sufficient statistics $T_{\mathrm{ER}}(g)$.  
Given a graph $g$, we know that $g$ has at least $0$ edges between the nodes in block $B_i$ and the nodes in block $B_j$ for any choice of $i$ and $j$.  
We also know that $g$ has no more than $n_in_j$ edges between the nodes in block $B_i$ and $B_j$ for $i\neq j$, and no more than ${n_i\choose 2}$ edges between the nodes of block $B_i$.  
Thus, $0\leq T_{\mathrm{ER}}(g)_{ij}\leq n_in_j$ if $i\neq j$ and $0\leq T(g)_{ii}\leq {n_i\choose 2}$ for all $i\in[k]$.  
Therefore, $P_{\M_{\mathrm{ER}}}\subseteq P$.  
\end{proof}

\smallskip 
Next we derive a Markov basis for the model. As stated in Section 5, this is done using an identification--standard in algebraic statistics--between odds (or log-odds) of  dyad probabilities  and algebraic indeterminates. Then, one uses the model parametrization to construct an algebraic map between two polynomial rings. The kernel of this map is a polynomial ideal, any generating set of which is a Markov basis of the model by \cite[Theorem 3.1]{DS98}. 

The  model parametrization map is encoded algebraically as follows.  There are two sets of indeterminates in the map:  $x_{uv}$ and $t_{ij}$.  The indeterminates $x_{uv}$  represent $\frac{p_{uv}}{1-p_{uv}}$, the odds of the edge probabilities of the edge $\{u,v\}$ appearing in the random graph.  
The indeterminates $t_{ij}$ represent  the model parameters $\alpha_{ij}$ via $t_{ij}=e^{\alpha_{ij}}$. 
Let $K$ denote some field of coefficients, say $K=\mathbb Q$. We construct the following semigroup algebra homomorphism:
\begin{equation*}
\begin{split}
\varphi_{\mathrm{ER}}&: K[x_{uv} : 1\leq u<v\leq n] \longrightarrow K[t_{ij}: 1\leq i\leq j\leq k];\\
\varphi_{\mathrm{ER}}&: x_{uv} \longmapsto t_{z(u)z(v)}.\\
\end{split}
\end{equation*}
To recover  exactly the model parametrization from the map $\varphi_{ER}$, simply interpret $x_{uv}=\frac{p_{uv}}{1-p_{uv}}$ and $t_{ij}=e^{\alpha_{ij}}$ in the mapping $x_{uv}\mapsto t_{z(u)z(v)}$ to obtain: 
%~\eqref{erSBM}. 
\begin{eqnarray*}%\label{erSBM}
 \log \left(\frac{p_{uv}}{1-p_{uv}}\right)\mapsto \alpha_{z(u)z(v)} .
 \end{eqnarray*}
 
 The ideal of the model encoding the Markov bases is the kernel of this polynomial map. In algebraic terms, the toric ideal $I_{\M_\mathrm{ER}}$ associated to an ER-SBM $\M_{\mathrm{ER}}$ is the kernel of this semigroup algebra homomorphism, $I_{\M_\mathrm{ER}} :=\ker(\varphi_{\mathrm{ER}})$.  
Elements in this toric ideal are binomials  of the form such as  $x_{uv}-x_{yw}$. Each such binomial corresponds to a Markov move in the following way: it instructs one to move from a graph $g$ containing the edge $\{u,v\}$ but not the edge $\{y,w\}$ to a graph $h$ containing the edge $\{y,w\}$ but not the edge $\{u,v\}$.  
In Theorem A.2, we derive a set larger than a minimal Markov basis, called a Graver basis, and then extract a Markov basis from it. The definition of Graver is within the proof below. 

\smallskip
%---THEOREM: Graver Basis for ER-SBM----
%\begin{theorem}
\noindent{\bf Theorem A.2}\label{thm: graver basis for ER-SBM}
\emph{
Let $\M_{\mathrm{ER}}$ be an ER-SBM with associated toric ideal $I_{\M_{\mathrm{ER}}}$.  
The Graver basis of $\M_{\mathrm{ER}}$ is 
$$
\Gr_{\M_{\mathrm{ER}}} := \{x_{uv}-x_{yw} : u,y\in B_i; v,w\in B_j, \mbox{ and } i,j\in[k]\}.
$$
Moreover, a Markov basis for $\M_{\mathrm{ER}}$ consists of replacing any edge between blocks $B_i$ and $B_j$ for $i,j\in[k]$ with any other edge connecting the same blocks.  
}
%\end{theorem}
\begin{proof}

Given a nonnegative integer vector $m=(m_1,\ldots,m_N)\in\Z^N$, we let $x^m:=x_1^{m_1}x_2^{m_2}\cdots x_N^{m_N}$.  
Recall that any integer vector $u\in\Z^N$ can be written uniquely as $u = u^+-u^-$ where $u^+$ and $u^-$ are nonnegative integer vectors with disjoint support.  
We let $\Phi$ denote the sublattice of $\Z^{n\choose 2}$ consisting of all vectors $u$ such that $\varphi(x^{u^+}) = \varphi(x^{u^-})$.  
If $\M$ is any log-linear statistical model and if $\varphi$ is the associated semigroup homomorphism,
it is a fundamental result in toric geometry that $I_\M = \langle x^{u^+}-x^{u^-} : u\in\Phi\rangle$; see \cite[Corollary 4.3]{St}.  
A binomial $x^{u^+}-x^{u^-}\in I_\M$ is called \emph{primitive} if there exists no other binomial $x^{v^+}-x^{v-}\in I_\M$ such that $x^{v^+}\mid x^{u^+}$ and $x^{v^-}\mid x^{u^-}$.  
The \emph{Graver basis} of $I_\M$ is a generating set for $I_\M$ consisting of all primitive binomials in $I_\M$, and we denote it by $\Gr_\M$.  

By the definition of the toric ideal $I_{\M_{\mathrm{ER}}}$ it is straight-forward to see that the primitive binomials in $I_{\M_{\mathrm{ER}}}$ are precisely the linear forms given above.  
The description of the Markov basis is then immediate from the definition of $I_{\M_{\mathrm{ER}}}$, and its existence follows from \cite[Theorem 3.1]{DS98}.  
\end{proof}

\section*{Appendix B:  Algebraic and geometric proofs of structure of the  additive SBM}

This section describes the additive SBM polytope and Markov basis. 
The $H$-representation for the additive SBM model polytope given in Theorem  5.5. %~\ref{thm: additive SBM model polytope} 
 explicitly generalizes that of the $\beta$-model, and the proof of this theorem follows analogously.  

\smallskip
%Theorem B.1. is identical to Theorem  5.5., re-stated here for completeness. 
%---THEOREM: Additive SBM Model Polytope H-representation----
%\begin{theorem}
%\label{thm: additive SBM model polytope}
\noindent {\bf Theorem B.1. [Theorem 5.5.]}
Let $\M_{\mathrm{Add}}$ be an additive SBM model defined on node set $[n]$ with block structure $\B := \{B_1,\ldots,B_k\}$.
Let $T,S\subset\B$ be such that 
\begin{equation}
\label{eqn: subset conditions appendix}
T\cup S \neq \emptyset 
\qquad
\mbox{and}
\qquad
T\cap S = \emptyset.  
\end{equation}
The model polytope $P_{\M_{\mathrm{Add}}}$ is the intersection of the closed halfspaces defined by the inequalities
\begin{equation}
\label{eqn: additive sbm inequalities appendix}
\sum_{B_i\in T} x_i - \sum_{B_i\in S} x_i 
\leq 
2{\sum_{B_i\in T}n_i\choose 2} + \sum_{ \substack{B_j \in \mathbb{B} \setminus (T\cup S) \\ B_i \in T} }n_in_j,
\end{equation}
ranging over all such pairs of subsets of $\B$.  
%\end{theorem}

We will  present a proof of Theorem 5.5. %~\ref{thm: additive SBM model polytope} 
for the sake of completeness.  
To do so, we first prove the following short lemma.  

\smallskip
%---LEMMA: Additive SBM Model Polytope Lemma-----
%\begin{lm}
\noindent{\bf Lemma B.1.}
\label{lem: additive SBM model polytope}
\emph{
Let $S$ and $T$ be subsets of $\B$ satisfying the conditions in  \eqref{eqn: subset conditions appendix}.  
Then inequality \eqref{eqn: additive sbm inequalities appendix}
 is valid for the model polytope $P_{\M_{\mathrm{Add}}}$.  
Moreover, the sufficient statistics of a graph $g$ satisfy \eqref{eqn: additive sbm inequalities appendix} 
with equality if and only if the following hold.
\begin{enumerate}[(i)]
	\item The nodes within blocks of $T$ form a clique in $g$.
	\item The nodes within blocks of $S$ form an independent set in $g$. 
	\item Every node in blocks within $T$ is adjacent to all nodes in blocks in $\B\setminus(T\cup S)$, and
	\item Every node in blocks within $S$ is not adjacent to any node in $\B\setminus(T\cup S)$.  
\end{enumerate}
}
%\end{lm}
\begin{proof}
Let $T_{\mathrm{Add}}(g) = (T_{\mathrm{Add}}(g)_1,\ldots,T_{\mathrm{Add}}(g)_k)$ denote the additive SBM sufficient statistics of the graph $g$.  
We claim that the following inequality holds:
$$
\sum_{B_i\in T} T_{\mathrm{Add}}(g)_i 
\leq 
2{\sum_{B_i\in T}n_i\choose 2} + \sum_{ \substack{B_j \in \mathbb{B} \setminus (T\cup S) \\ B_i \in T} }n_in_j + \sum_{B_i\in S} T_{\mathrm{Add}}(g)_i.
$$
To see this, notice that the first term on the right-hand-side double counts the maximum number of edges that can exist amongst nodes in blocks within $T$.  
Similarly, the second term counts the maximum number of edges that can exist between nodes in blocks within $T$ and nodes in blocks within $\B\setminus(T\cup S)$.  
Thus, to bound the total degree of nodes in blocks within $T$, it only remains to bound the number of edges between nodes in blocks within $T$ and nodes in blocks within $S$.  
This bound is given by the third term on the right-hand-side.  
Thus, inequality \eqref{eqn: additive sbm inequalities appendix}
 is valid for $P_{\M_{\mathrm{Add}}}$.   
The characterization of when equality occurs is clear from the above proof.
\end{proof}

The following proof of the theorem parallels that for the polytope of degree sequences as presented in \cite[Chapter 3]{MP95}.  

%---SUBSUBSECTION: Proof of Theorem~\ref{thm: additive SBM model polytope}-----
%\sub

\begin{proof}[Proof of Theorem B.1]
%\label{subsubsec: proof of additive SBM H-representation}
Let $P$ be the polytope determined by the inequalities (12). %  (\ref{eqn: additive sbm inequalities}).  
By Lemma~B.1, %\ref{lem: additive SBM model polytope}, 
we know that $P_{\M_{\mathrm{Add}}}\subseteq P$.  
So it only remains to show that $P\subseteq P_{\M_{\mathrm{Add}}}$.  
To do this, we can show that for a cost vector $c^T = (c_1,\ldots,c_k)^T\in\R^k$ the linear program
\begin{equation}
\label{prgm: model polytope}
\begin{split}
\mbox{maximize}& 
\qquad c^Tx	\\
\mbox{subject to}&
\qquad 
x\in P_{\M_{\mathrm{Add}}}	\\
\end{split}
\end{equation}
has the same optimum solution as 
\begin{equation}
\label{prgm: H-representation}
\begin{split}
\mbox{maximize}& 
\qquad c^Tx	\\
\mbox{subject to}&
\qquad 
x\in P.	\\
\end{split}
\end{equation}
Notice first that producing an optimal solution $x^\ast$ to (\ref{prgm: model polytope}) is easy.  
Recall that our graphs all have node set $[n]$ partitioned into $k$ nonempty blocks $\B = \{B_1,\ldots, B_k\}$, and that each block $B_i$ is associated to a coordinate-value $c_i$ of the cost vector $c$.  
So we construct an optimal graph $g^\ast$ on node set $[n]$ as follows: for every pair of nodes $\{u,v\}\subset{[n]\choose 2}$, if $c_i+c_j\geq 0$ then add the edge $\{u,v\}$ to $g^\ast$.  
Let $T(g^\ast) =: x^\ast$ denote the sufficient statistics of $g^\ast$.  
It remains to show that $x^\ast$ is an optimal solution to (\ref{prgm: H-representation}).  
The dual linear program to (\ref{prgm: H-representation}) can be formulated as 
\begin{equation}
\label{prgm: dual H-representation}
\begin{split}
\mbox{minimize}& 
\qquad \sum_{
\substack{T,S \subset\mathbb{B} : \\ 
T\cup S \neq \emptyset, \\
T\cap S = \emptyset	\\}}
\left(
2{\sum_{B_i\in T}n_i\choose 2} + \sum_{ \substack{B_j \in \mathbb{B} \setminus (T\cup S) \\ B_i \in T} }n_in_j
\right)
y_{T,S}\\
\mbox{subject to}&
\qquad 
\sum_{B_i\in T}x_i - \sum_{B_j\in S} x_i = c_i \mbox{ and } x_i\geq 0.	\\
\end{split}
\end{equation}
By complementary slackness, whenever the primal variable $y_{T,S}>0$ then the corresponding dual inequality must be tight.  
That is, whenever $y_{T,S}>0$ then
\begin{equation}
\label{eqn: tightness}
\sum_{B_i\in T} x_i - \sum_{B_i\in S} x_i 
= 
2{\sum_{B_i\in T}n_i\choose 2} + \sum_{ \substack{B_j \in \mathbb{B} \setminus (T\cup S) \\ B_i \in T} }n_in_j,
\end{equation}
Thus, to show that $x^\ast$ is optimal with respect to (\ref{prgm: H-representation}), it suffices to produce a dual solution $y$  such that $y_{T,S}>0$ only when (\ref{eqn: tightness}) holds.  

To do this, we first reindex the blocks of $\B$ such that 
$$
c_1\leq c_2\leq \cdots \leq c_r < 0 \leq c_{r+1} \leq \cdots \leq c_k.
$$
Then it is clear that, for the graph $g^\ast$, the nodes within blocks $B_1,\ldots, B_r$ form a stable set, and the nodes within blocks $B_{r+1},\ldots, B_k$ form a clique.  
Moreover, by the construction of $g^\ast$, we have that
\begin{equation}
\label{eqn: optimal graph observations}
\begin{split}
N(B_1)\subseteq N(B_2)\subseteq&\cdots\subseteq N(B_r), \mbox{ and} \\
N(B_{r+1})\cap\{v\in[n] : v\in B_i, i\in[r]\}\subseteq&\cdots\subseteq N(B_k)\cap\{v\in[n] : v\in B_i, i\in[r]\},\\
\end{split}
\end{equation} where $N(B_i)$ denotes the neighborhood of the block $B_i$.
We now construct the following pairs of subsets of $\B$: 
For all $i\in[r]$ define
\begin{equation}
\begin{split}
T_i &:= \{B_j : \exists u\in B_i \mbox{ and } v\in B_j \mbox{ such that } \{u,v\}\in E(g^\ast)\}, \mbox{ and}	\\
S_i &:= \{B_1,\ldots, B_k\}.	\\
\end{split}
\end{equation}
Then for all $i\in[k]\setminus[r]$ define 
\begin{equation}
\begin{split}
T_i &:= \{B_i,\ldots, B_k\}, \mbox{ and}	\\
S_i &:= \{B_1,\ldots,B_r\}\setminus\{B_j : \exists u\in B_i \mbox{ and } v\in B_j \mbox{ such that } \{u,v\}\in E(g^\ast)\}. 	\\
\end{split}
\end{equation}
It follows from the observations (\ref{eqn: optimal graph observations}) and Lemma~\ref{lem: additive SBM model polytope} that each pair $(T_i,S_i)$ satisfies (\ref{eqn: additive sbm inequalities appendix}) with equality.  
Thus, our goal is to find a feasible solution $y^\ast$ such that $y_{T,S}>0$ only if $(T,S) = (T_i,S_i)$ for some $i$.  

Since $T_i\subset\{B_{r+1},\ldots, B_k\}$, and $S_i\subset\{B_1,\ldots,B_r\}$, then we may rewrite the dual feasibility conditions as 
\begin{equation}
\label{eqn: rewritten dual feasibility conditions}
\begin{split}
\sum_{i : B_j\in S_i}y_{T_i,S_i} &= |c_j| \mbox{ for all $j\in[r]$,}	\\
\sum_{i : B_j\in T_i}y_{T_i,S_i} &= |c_j| \mbox{ for all $j\in[k]\setminus[r]$, and }	\\
y_{T_i,S_i}&\geq 0.	\\
\end{split}
\end{equation}
We must now show that these equations have a nonnegative solution.  

For each $j\in[k]$, let $P_j$ denote the set of indices $i$ such that $y_{T_i,S_i}$ appears in the $j^{th}$ equation for (\ref{eqn: rewritten dual feasibility conditions}).  
Then for $j\in[r]$,
\begin{equation*}
\begin{split}
P_j
&= \{i\in[k] : B_j\in S_i\}, 	\\
&= \{i\in[r] : i\geq j\}\cup\{i\in[k]\setminus[r]: \forall u\in B_i, v\in B_j, \{u,v\}\notin E(g^\ast)\},		\\
&= \{i\in[r] : i\geq j\}\cup\{i\in[k]\backslash[r] : c_i < |c_j|\},		\\
&= \{i\in[r] : i\geq j\}\cup\{i\in[k]\backslash[r] : |c_i| < |c_j|\}.		\\
\end{split}
\end{equation*}
Similarly, for $j\in[k]\backslash[r]$, we have that
$$
P_j = \{i\in[k]\backslash[r] : i\leq j\}\cup\{i\in[r]: |c_j|\geq|c_i|\}.
$$
Let $\pi = \pi_1\ldots\pi_k$ be permutation of $[k]$ that sorts the components of $c$ by nondecreasing absolute values, resolving ties as follows: 
\begin{enumerate}
	\item $|c_{\pi_1}|\leq |c_{\pi_2}|\leq \cdots\leq|c_{\pi_k}|$;
	\item If $|c_{\pi_i}| = |c_{\pi_j}|$ for some $i\neq j$ then 
	$$
	\begin{cases}
		(i-j)(\pi_i-\pi_j)<0	&	\mbox{ if $\pi_i,\pi_j\in[r]$},	\\
		(i-j)(\pi_i-\pi_j)>0	&	\mbox{ if $\pi_i,\pi_j\in[k]\setminus[r]$},	\\
		\pi_i<\pi_j			&	\mbox{ if $\pi_i\in[r]$ and $\pi_j\in[k]\setminus[r]$}.\\
	\end{cases}
	$$
\end{enumerate}
We then have that $P_{\pi_j} = \{\pi_1,\ldots,\pi_j\}$.  
Therefore, applying the permutation $\pi^{-1}$ to the index order of the equations (\ref{eqn: rewritten dual feasibility conditions}) and to the index order of the variables $y_{T_i,S_i}$ produces a system $Ay = b$ in which $A$ has zeros above the diagonal and ones everywhere else.  
Since the values of $b$ are all nonnegative, this system has the desired nonnegative solution. 
This completes the proof. % \hfill$\square$
\end{proof}

%\subsection*{Additive SBM  Markov basis}
\smallskip 

%Our next goal is to compute a Markov basis for the additive SBM. 
Similar to the case of the ER-SBM, Markov basis derivation can be accomplished using techniques from toric algebra.  
As before, the algebraic object corresponding to the statistical model is defined using a map which essentially encodes the model parametrization: again, the indeterminates $x_{uv}$ correspond to the log-odds of the edge probabilities, that is, setting $x_{uv}=\frac{p_{uv}}{1-p_{uv}}$ and $t_i=e^{\alpha_i}$ recovers the model parametrization:% from Equation~\eqref{addSBM} 
\begin{eqnarray*}%\label{addSBM}
\log \left(\frac{p_{uv}}{1-p_{uv}}\right)  =\alpha_{z(u)} + \alpha_{z(v)}.
\end{eqnarray*}
%{\color{red} THIS SEEMS TO BE REFERRING TO MAIN TEXT. REWRITE and unify explanations that are trying to "make alg stats intuitive"!! $\rightarrow$ See also explanations and illustrations following the next Theorem. } 
Markov moves derived from this section are illustrated by an example in Figure 2 in the main text. 
%\textcolor{cyan}{HOLD UP: I wanted to change the $t$s to the $\alpha$s from the model parametrization, like I did for the ER-SBM; but that's abuse of notation! In reality, we do an extra step: $x_{uv}$ equals the odds, not log-odds, of edge probabilities; then we take logs and addition becomes multiplication on the parameter side. So really $t_i=e^{\alpha_i}$, and $x_{uv}=\frac{p_{uv}}{1-p_{uv}}$. Need to make the edit in the ER-SBM too. Just call the parameters $t$s in this section and then we will be consistent and not hide any details! --Sonja will edit.}
In this case, the toric ideal associated to $\M_{\mathrm{Add}}$ is defined by the semigroup algebra homomorphism 
\begin{equation*}
\begin{split}
\varphi_{\mathrm{Add}}&: K[x_{uv} : 1\leq u<v\leq n] \longrightarrow K[t_1,\ldots,t_k];\\
\varphi_{\mathrm{Add}}&: x_{uv} \longmapsto t_{z(u)}t_{z(v)}.\\
\end{split}
\end{equation*}
We denote this toric ideal by $I_{\M_{\mathrm{Add}}}:=\ker(\varphi_{\mathrm{Add}})$.  
The algebra of this toric ideal is intimately described by the relationship between the $\beta$-model and the additive SBM model.  
The toric ideal for the typical $\beta$-model is the kernel of the semigroup algebra homomorphism
\begin{equation*}
\begin{split}
\rho&: K[x_{uv} : 1\leq u<v\leq n] \longrightarrow K[\beta_1,\ldots,\beta_n];\\
\rho&: x_{uv} \longmapsto \beta_u\beta_v,\\
\end{split}
\end{equation*}
and we denote it by $I:=\ker(\rho)$.  
It is a well-known fact that $I$ is a toric ideal of the Veronese-type corresponding to the $(n,2)$-hypersimplex.  
The toric ideal $I_{\M_{\mathrm{Add}}}$ arises from applying the linear map
\begin{equation*}
\begin{split}
\tau&:K[\beta_1,\ldots,\beta_n]\longrightarrow K[t_1,\ldots,t_k];\\
\tau&:\beta_i\longmapsto t_{z(i)}
\end{split}
\end{equation*}
to the toric ideal $I$.  
That is to say, $I_{\M_{\mathrm{Add}}} = \ker(\tau\circ\rho)$, and consequently, any Markov basis for the $\beta$-model can be extended to a basis for the additive SBM model via the addition of some linear forms to its corresponding binomial generating set.  

A famous and well-investigated binomial generating set for a variety of the Veronese-type is a quadratic and \emph{reduced Gr\"obner basis} \cite{St} known in the literature as the \emph{sorted basis} or \emph{sort-closed basis} and it is described in detail in \cite[Chapter 14]{St}.   
In the case of the $(n,2)$-hypersimplex and its associated toric ideal $I$, this reduced Gr\"obner basis arises from a completely lexicographic term order, and its binomials correspond to special $4$-cycles in the complete graph $K_n$ \cite[Chapter 9]{St}.  
We denote this Gr\"obner basis for $I$ by $\mathcal{G}$.  

\smallskip 
%---THEOREM: Markov Basis for Additive SBM------
%\begin{theorem}
\noindent{\bf Theorem B.2}
\label{thm: markov basis for additive SBM}
\emph{
Let $\M_{\mathrm{Add}}$ be an additive SBM model with associated toric ideal $I_{\M_{\mathrm{Add}}}$, and let $\mathcal{G}$ denote the sorted basis for the toric ideal of the $(n,2)$-hypersimplex.  
Then 
$$
\mathcal{G}\cup\{x_{uv}-x_{yw} : u,y\in B_i; v,w\in B_j, \mbox{ and } i,j\in[k]\}
$$
is a Gr\"obner basis for $I_{\M_{\mathrm{Add}}}$.  
Moreover, a Markov basis for $\M_{\mathrm{Add}}$ is given by an exchange of edges along any sorted $4$-cycle and the exchange of any edge for any other edge whose endpoints lie in the same respective blocks.  
}
%\end{theorem}
\begin{proof}
By \cite[Lemma 5.1]{NP08} the proposed collection of binomials is a Gr\"obner basis for $I_{\M_{\mathrm{Add}}}$.  
The description of the associated Markov basis follows from the description of the sorted basis of $I$ in \cite[Chapter 9]{St}, and its existence is immediate from \cite[Theorem 3.1]{DS98}.  
\end{proof}

Similar to Theorem~A.2, Theorem~B.2 %\ref{thm: graver basis for ER-SBM}, Theorem~\ref{thm: markov basis for additive SBM} 
 allows us to identify a Markov basis as follows. 
The indeterminate $x_{uv}$ corresponds to the odds of the probability $p_{uv}$ of the edge $\{u,v\}$ appearing in the graph.  
As noted following Theorem~4.5 in the paper, %\ref{thm: corollary to markov basis theorem for additive SBM}, 
 this Markov basis contains the same moves as the ER-SBM plus the additional moves that corresponding to switching edges along a $4$-cycle.

%Similar to Theorem~\ref{thm: graver basis for ER-SBM}, Theorem~\ref{thm: markov basis for additive SBM} allows us to identify a Markov basis.  
%Just as before, the indeterminate $x_{uv}$ corresponds to the odds of the probability $p_{uv}$ of the edge $\{u,v\}$ appearing in the graph.  
%\textcolor{red}{start of repeated text:} 
%In this Markov basis, we now have the same moves as the ER-SBM, but also a collection of ``quadratic" moves corresponding to switching edges along a $4$-cycle.    
%For example, the binomial $x_{uv}x_{yw}-x_{uy}x_{vw}$ for $u,w\in B_i$ and $v,y\in B_j$ corresponds to a move from a graph $g$ containing the two edges $\{u,v\}$ and $\{y,w\}$ but not the edges $\{u,y\}$ and $\{v,w\}$ to a graph $h$ containing the edges $\{u,y\}$ and $\{v,w\}$ but not the edges $\{u,v\}$ and $\{y,w\}$.  
%Collectively, the four edges $\{u,v\}, \{y,w\}, \{u,y\}$ and $\{v,w\}$ form a $4$-cycle.  
%An example of one such move was depicted in Figure~\ref{fig: markov basis for additive SBM}.
%\textcolor{red}{end of repeated text.} 

%\subsection{
\section*{Appendix C:  Algebraic and geometric proofs of structure of the $\beta$-SBM model}

Proposition~5.7,  %\ref{prop: beta-SBM model polytope}, 
restated here as Proposition~C.1, states the structure of the $\beta$-SBM polytope. 
%---PROPOSITION: beta-SBM Model Polytope----
%\begin{prop}

\smallskip
{\bf Proposition C.1. [Proposition 5.7.]} 
\emph{
Let $\B = \{B_1,\ldots,B_k\}$ be a partition of the node set $[n]$ into $k$ nonempty blocks.  
Let $\M_\beta$, $\M_{\mbox{\tiny ER}}$, and $\M$ respectively denote the $\beta$-SBM, ER-SBM, and $\beta$-models with respect to $\B$ and $[n]$.  
The model polytope $P_{\M_{\beta}}$ of the $\beta$-SBM is the free sum 
$$
P_{\M_{\beta}} = P_{\M_{\mbox{\tiny ER}}}\oplus P_{\M}.
$$
}
%\end{prop}
 
 \begin{proof} 
Let $P\subset\R^n$ be an $n$-dimensional convex polytope and let $Q\subset\R^m$ be an $m$-dimensional convex polytope.  
The \emph{free join} of $P$ and $Q$, denoted by $P\ovee Q$, is the $(n+m+1)$-dimensional polytope given by respectively embedding $P$ and $Q$ into skew affine spaces and taking their convex hull.  
For instance, 
$$
P\ovee Q := \conv(\{(p,0,0)\in\R^n\times\R^m\times\R : p\in P\}\cup\{(0,q,1)\in\R^n\times\R^m\times\R : q\in Q\}).
$$
The \emph{free sum} of $P$ and $Q$, denoted by $P\oplus Q$, is the projection of $P\ovee Q$ on $\R^n\times\R^m$ along the final coordinate of $\R^n\times\R^m\times\R$.  
The facets of $P\ovee Q$ are given by the joins of the $i$-faces of $P$ and the $(n+m-i-1)$-faces of $Q$ as $i$ varies over $-1,0,1,\ldots,n+m-1$.  
Using Fourier-Motzkin elimination on the collection of facet-supporting hyperplanes of $P\ovee Q$, one can recover a (redundant) $H$-representation of $P\oplus Q$.  
For more details on these combinatorial operations see \cite{HRGZ95,K88} and \cite[Chapter 1]{Z95}.  
The claim %Proposition~\ref{prop: beta-SBM model polytope} 
 then follows immediately.  
A valid $H$-representation of $P_{\M_{\beta}}$ is then given by applying Fourier-Motzkin elimination to the $H$-representation of the free join $P\ovee Q$.  
\end{proof} 

{\bf An open problem: Markov basis for $\beta$-SBM.} 
%{\color{magenta} spell out - it is an open problem!} 
It remains to describe how we can recover a Markov basis for the $\beta$-SBM model.  
Theoretically, the desired Markov basis is encoded in any binomial generating set for the toric ideal that is the kernel of the following semigroup algebra homomorphism:
%\textcolor{cyan}{to do (sonja): this is now abuse of notation. see previous 2 models. really, below, the $\alpha$s and $\beta$s are equal to $\exp(original parameters)$..}
\begin{equation*}
\begin{split}
%\varphi&: k[x_{uv} : 1\leq u<v\leq n] \longrightarrow k[\{\alpha_{st}: 1\leq s\leq t\leq k\}\cup\{\beta_1,\ldots, \beta_n\}];\\
%\varphi&: x_{uv} \longmapsto \alpha_{c(u)c(v)}\beta_u\beta_v.\\
\varphi_\beta&: K[x_{uv} : 1\leq u<v\leq n] \longrightarrow K[\{t_{ij}: 1\leq i\leq j\leq k\}\cup\{s_1,\ldots, s_n\}];\\
\varphi_\beta&: x_{uv} \longmapsto t_{z(u)z(v)}s_us_v,\\
\end{split}
\end{equation*}
where $z$ is the block assignment function as in the model definition. 
As before, the correspondence between this algebraic map and the statistical model parametrization is clear: the indeterminates $x_{uv}$ correspond to the odds of the edge probabilities and the $t_i$'s and $s_i$'s correspond to the model parameters; specifically, setting $x_{uv}=\frac{p_{uv}}{1-p_{uv}}$, $s_u=e^{\beta_u}$, and $t_{ij}=e^{\alpha_{ij}}$ recovers the model parametrization from Equation~(2): %\eqref{addSBM}.  
\begin{eqnarray*}%\label{addSBM}
\log \left(\frac{p_{uv}}{1-p_{uv}}\right)  =\alpha_{z(u)} + \alpha_{z(v)}.
\end{eqnarray*}

The Markov basis analyzed in Example~4.7 %\ref{ex: beta-SBM example} 
 is recovered by computing the kernel of the above semigroup algebra homomorphism using the software {\tt Macaulay2} \cite{M2}. Therefore, the results for any given example run are correct, even though we did not obtain a theoretical description for a Markov basis for an arbitrary number of nodes and blocks.
